# Supplementary material for: Orbits of very distant asteroid satellites
Source: arXiv:2503.15081 source file (2025-03-19)
Supplement: Supplementary file 1 [file appendix.tex]

abstract
